# Supplementary material for: In-Context Prompt Editing For Conditional Audio Generation
Source: arXiv:2311.00895 source file (2023-11-01)
Supplement: Supplementary file 1 [file appendix.tex]

\section{Appendix}

\subsection{Instruction-generating template}
\label{inst_template}

\begin{table*}[h]
    \centering
    \footnotesize
    \resizebox{\textwidth}{!}{
    \begin{tabular}{p{0.3\linewidth} p{0.2\linewidth}p{0.5\linewidth}}
\toprule
\textbf{User Input} & \textbf{ Instruction} & \textbf{Enhanced Prompt} \\
\midrule
\emph{Write a detailed description describing the music with instruments, tone, pitch, rhythm, atmosphere, style, and all the audio details.}

& \emph{Rewrite the following prompts to be diverse and different}

& \emph{1. Describe the instruments used in the music, including their tone, pitch, and rhythm. 2. Provide details about the overall sound and atmosphere of the music, including the style and genre. 3. Include any special effects or layers that enhance the music, such as layers of guitars or synths.} \\
% \hdashline
\bottomrule
\end{tabular}}
\caption{\small The provided example represents a pair of instruction-input and output generated by instruction-tuned LLMs.}\label{tab:example}
\end{table*}

\subsection{Sample generation}
\label{sample_gen}

% \begin{figure}[h]
%   \centering
% \includegraphics[width=1\columnwidth]{emnlp2023-latex/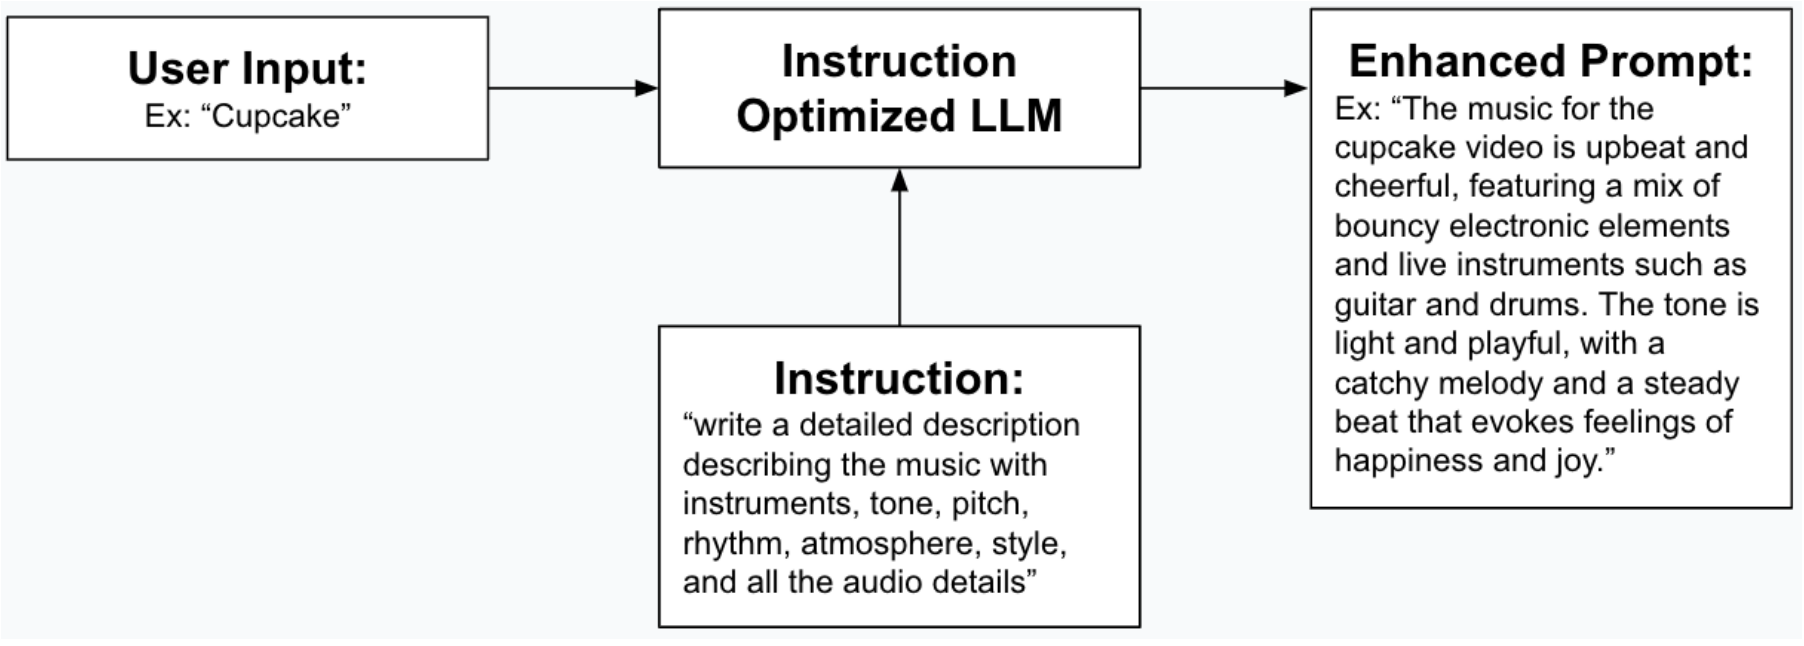}
% \caption{ \small  The provided example represents a pair of instruction-input and output that is utilized to train instruction-tuned LLMs.}
% \label{fig:example}
% \end{figure}

\begin{table*}[h]
    \centering
    \footnotesize
    \resizebox{\textwidth}{!}{
    \begin{tabular}{p{0.30\linewidth} p{0.70\linewidth}}
\toprule
\textbf{User Input} & \textbf{Enhanced Prompt (Instruct+Feedback)} \\
\midrule
% \emph{Cupcake}

% & \emph{The music for the cupcake video is upbeat and cheerful, featuring a mix of bouncy electronic elements and live instruments such as guitar and drums. The tone is light and playful, with a catchy melody and a steady beat that evokes feelings of happiness and joy.} \\

\emph{bumpy jazz}	&
\emph{The music is bumpy and jazzy.} \\ \hline
	
\emph{sad harp solo}	&
\emph{The harp solo is sad and haunting.} \\ \hline

\emph{cozy warm hip hop beat}	&
\emph{a hip hop beat with a warm atmosphere} \\\hline

\emph{fashion upbeat}	&
\emph{The music is upbeat and energetic.} \\\hline

\emph{gnarly beats that are fast and crazy}	&
\emph{a sonic journey} \\ 

% \hdashline
\bottomrule
\end{tabular}}
\caption{\small The provided example represents a pair of instruction-input and output that is utilized to train instruction-tuned LLMs.}\label{tab:example}
\end{table*}

% \subsection{Instruction Formats}
% \label{instruction}

% \input{emnlp2023-latex/sections/instruction_format}
% \input{emnlp2023-latex/sections/example}

\subsection{Training details}
% \subsection{Learning curve}

% \begin{figure}[h]
%   \centering
% \includegraphics[width=0.5\columnwidth]{emnlp2023-latex/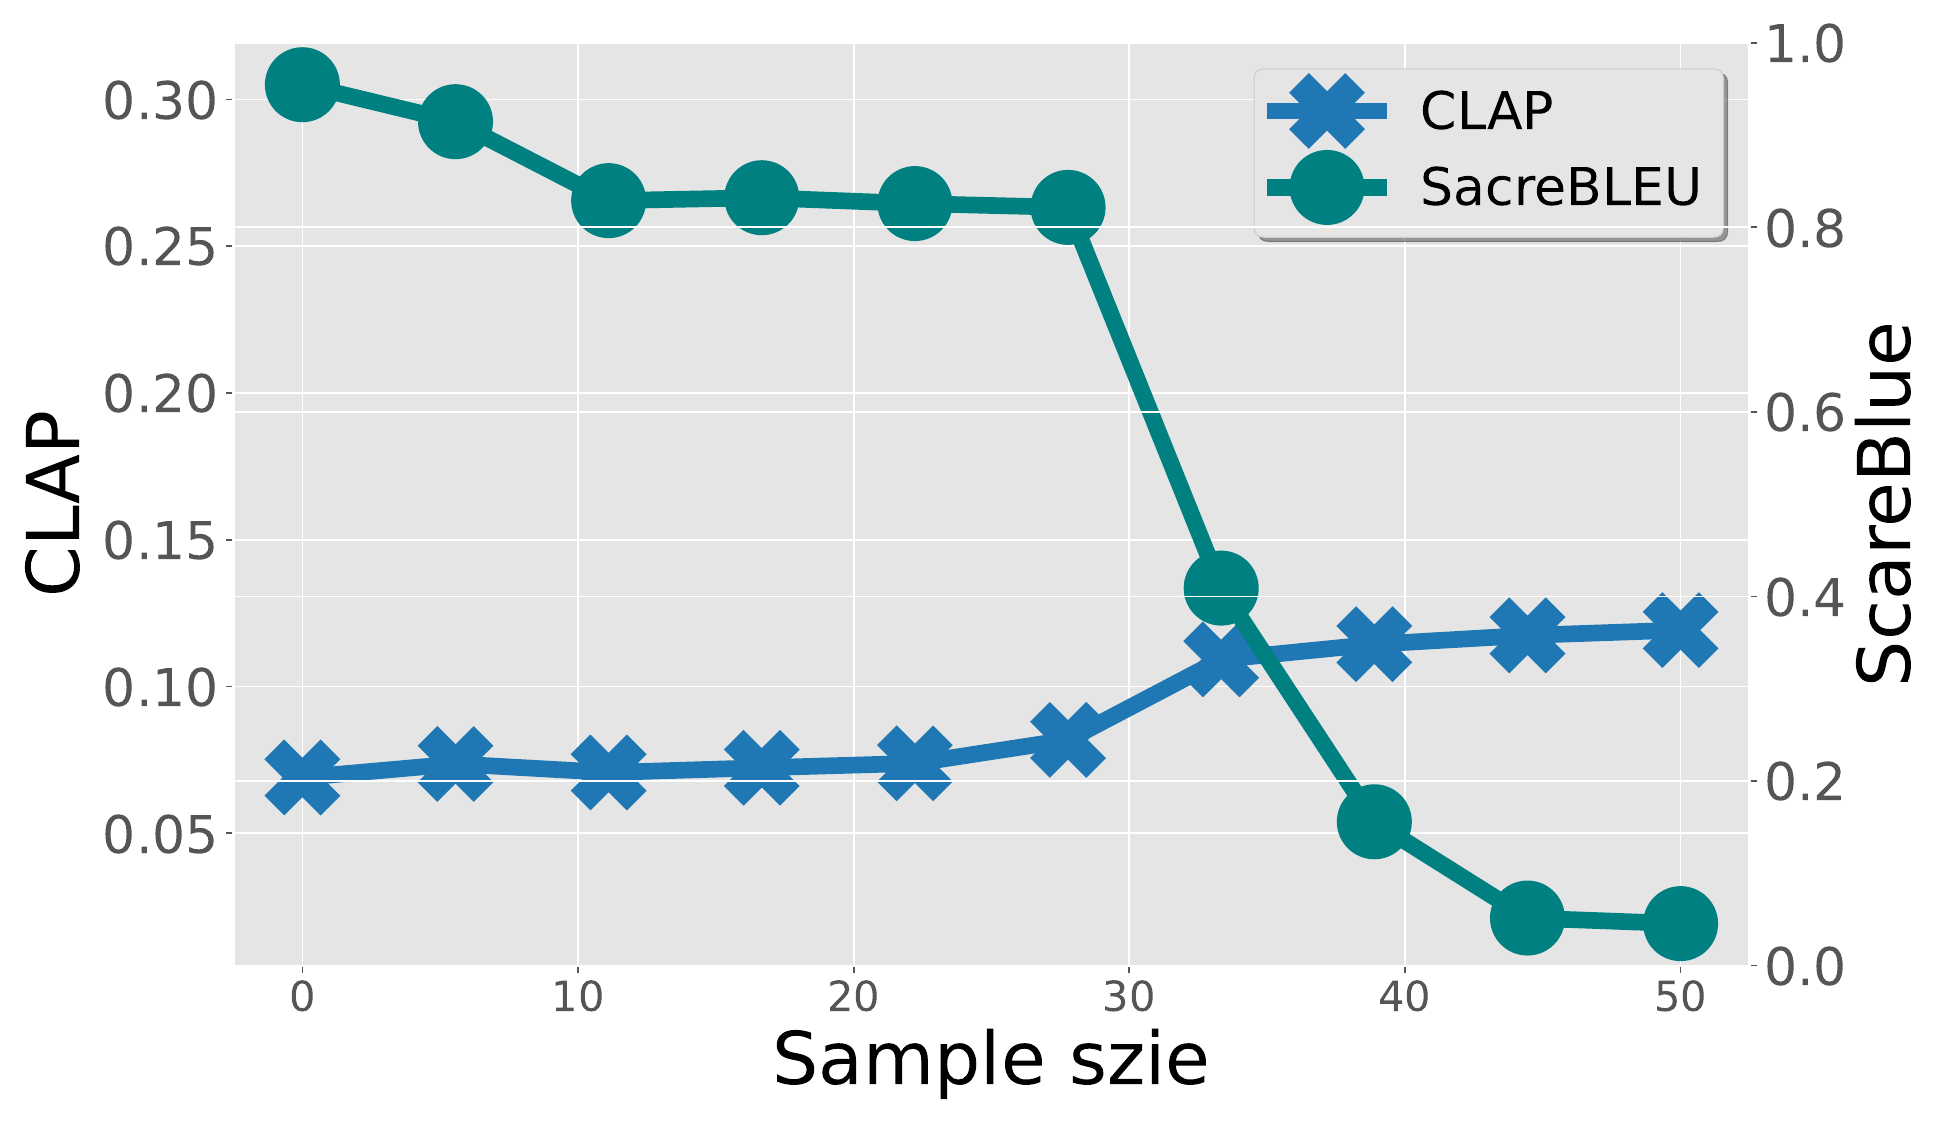}
% \caption{ \small \textbf{Learning curve:}
% The figure illustrates the learning curve at small sample size of $50$, with an iterval size of $5$.}
% \label{fig:learning_curve}
% \end{figure}

%We r show a learning curve, ranging from 0 to 350 at 10-sample intervals, providing insights into the impact of XXX.
\label{lr}

In practice, we found the margin rank learning process to be rather brittle. 
We set the learning rate to be 3e-4 and with training samples up to $50$ samples, and observed that the attained CLAP scores to go significantly higher as more samples are added, but at the huge cost of the text similarity with the original prompts. 
To avoid drastic deviation from the original user intent (and hence the objective human evaluation), we pick lower training sample sizes between $5$-$10$, depending on the SacreBLEU threshold, and stop training when SacreBLEU goes below $20$ points. 
We summarize the relationship between SacreBLEU and CLAP below in Figure~\ref{fig:learning_curve}.

\begin{figure}[h]
  \centering
\includegraphics[width=0.5\columnwidth]{emnlp2023-latex/diagrams/fig_learning_curve.pdf}
\caption{ \small \textbf{Learning curve:}
The figure illustrates the learning curve at small sample size of $50$, with an iterval size of $5$.}
\label{fig:learning_curve}
\end{figure}
