# Supplementary material for: In-Context Prompt Editing For Conditional Audio Generation
Source: arXiv:2311.00895 source file (2023-11-01)
Supplement: Supplementary file 2 [file appendix_line_chart.tex]

% \begin{figure}[h]
%   \centering
% \includegraphics[width=0.5\columnwidth]{emnlp2023-latex/diagrams/fig_learning_curve.pdf}
% \caption{ \small \textbf{Learning curve:}
% The figure illustrates the learning curve at small sample size of $50$, with an iterval size of $5$.}
% \label{fig:learning_curve}
% \end{figure}
